# Supplementary material for: Code-as-Monitor: Constraint-aware Visual Programming for Reactive and Proactive Robotic Failure Detection
Source: arXiv:2412.04455 source file (2025-03-21)
Supplement: Supplementary file 2 [file supp.tex]

% % CVPR 2025 Paper Template; see https://github.com/cvpr-org/author-kit

% \documentclass[10pt,twocolumn,letterpaper]{article}

% %%%%%%%%% PAPER TYPE  - PLEASE UPDATE FOR FINAL VERSION
% % \usepackage{cvpr}              % To produce the CAMERA-READY version
% \usepackage[review]{cvpr}      % To produce the REVIEW version
% % \usepackage[pagenumbers]{cvpr} % To force page numbers, e.g. for an arXiv version

% % Import additional packages in the preamble file, before hyperref
% \input{preamble}

% % It is strongly recommended to use hyperref, especially for the review version.
% % hyperref with option pagebackref eases the reviewers' job.
% % Please disable hyperref *only* if you encounter grave issues, 
% % e.g. with the file validation for the camera-ready version.
% %
% % If you comment hyperref and then uncomment it, you should delete *.aux before re-running LaTeX.
% % (Or just hit 'q' on the first LaTeX run, let it finish, and you should be clear).
% \definecolor{cvprblue}{rgb}{0.21,0.49,0.74}
% \usepackage[pagebackref,breaklinks,colorlinks,allcolors=cvprblue]{hyperref}

% \usepackage{tabularx} % 引入tabularx宏包
% \usepackage{multirow} % 确保multirow宏包也被引入
% \usepackage{booktabs}
% \usepackage{amsmath}  
% \usepackage{amssymb}  
% \usepackage{mathrsfs} 
% \usepackage{amsthm,amsfonts}
% % \usepackage{cleveref}
% \usepackage{array}
% \usepackage{float}
% \usepackage{pifont} % \ding{xx}
% \usepackage{bbding} % \Checkmark,\XSolid,...
% \usepackage{fontawesome} % \faCheck,\faTime
% \def\ie{\emph{i.e.}}
% \def\eg{\emph{e.g.}}
% \def\etal{{\em et al.}}
% \def\etc{{\em etc.}} 
% \usepackage[dvipsnames]{xcolor}
% \newcommand{\mname}{\textsl{ConSeg}}
% \newcommand{\fname}{\textsl{CaM}}
% \definecolor{ourpurple}{HTML}{7030A0} 
% \definecolor{ouryellow}{HTML}{F4B402} 
% % \newcommand{\todo}[1]{{\color{red}#1}}
% % \newcommand{\update}[1]{{\color{orange}#1}}
% \newcommand{\highlight}[1]{\textbf{\color{ourpurple}#1}}
% % \newcommand{\highlight}[1]{\colorbox{yellow}{#1}}

% %%%



% %%%%%%%%% PAPER ID  - PLEASE UPDATE
% \def\paperID{786} % *** Enter the Paper ID here
% \def\confName{CVPR}
% \def\confYear{2025}

% \begin{document}
% \appendix
% %%%%%%%%% TITLE - PLEASE UPDATE
% \title{Code-as-Monitor: Constraint-aware Visual Programming for \\ Reactive and Proactive Robotic Failure Detection}

% % \maketitle
% \maketitlesupplementary

% %%%%%%%%% MAIN TEXT

% \noindent The supplementary document is organized as follows:
% \newline
% \begin{itemize}


%     \item Sec.~\ref{supsec: implementation details}: Implementation Details of Painter, including data collection, training, and element pipeline details.
%     \newline
%     \item Sec.~\ref{supsec: environment configuration}: Environment Configuration, including environmental setups, control policies, and baseline details.
%     \newline
%     \item Sec.~\ref{supsec: evaluation details}: Evaluation Details, including detailed task definition, disturbances, and experimental results.
%     \newline
%     \item Sec.~\ref{supsec: more discussion}: Limitations and Future Work.
%     \newline
%     \item Sec.~\ref{supsec: more demonstrations and prompts}: More Demonstrations of {\fname}.
% \end{itemize}




% \section{Constraint Painter}
% \label{supsec: implementation details}
% In this section, we first describe the data collection and annotation process of the Constraint-aware Segmentation Dataset. Next, we present the training details of the proposed {\mname} model. Finally, it is followed by a detailed explanation of the Element Pipeline.

% \begin{figure*}[t]
% \centering
% \includegraphics[width=\linewidth]{fig/data_collection.pdf}
%    \caption{Dataset Collection Pipeline. Our data is sourced from BridgeData V2~\cite{li2022behavior}. The data collection process consists of three steps: \textbf{(1)} Using GPT-4o~\cite{achiam2023gpt} to decompose the task instruction based on the initial observation from the first frame of the trajectory, generating subgoals along with two types of constraints for each subgoal (\ie, constraints during execution and upon completion) and object-part associations. \textbf{(2)} Utilizing external references (\eg, gripper open/close states) to assign subgoals, constraints, and object-part associations to each frame. (3) Leveraging off-the-shelf models (\eg, Grounded SAM~\cite{ren2024grounded}, Semantic SAM~\cite{li2023semantic}) to generate instance- and part-level masks~(blue mask in this figure) automatically, followed by manual filtering to curate the final dataset. 
%    % 
%    }
% \label{fig: sup data collection}
% \end{figure*}

% \subsection{{\mname} Data Collection}
% To ensure broader coverage of scenarios and objects in our dataset, along with text-based instructions, we utilized the BridgeData V2 dataset~\cite{walke2023bridgedata}. This large and diverse dataset of robotic manipulation behaviors comprises $60,096$ trajectories collected across $24$ environments, encompassing $13$ distinct skills.

% %
% The dataset collection pipeline is shown in \cref{fig: sup data collection}. The entire process is divided into three stages, \ie, trajectory decomposition, assigning textual information, and dataset collection.
% First, we decompose each trajectory’s instruction and initial observation from BridgeData V2 into subgoals for each stage, along with the constraints upon completion, constraints during execution, the corresponding object-part associations and element type for each constraint. 
% Subfigure 1 in \cref{fig: sup data collection} illustrates a specific example, demonstrating the decomposition of the task ``Take cup off plate''.
% Notably, the third subgoal, ``Place the cup on the stove'', indicates that the initial observation ensures the decomposition process fully understands the task's contextual environment.
% During this process, we also obtain the constraint element type, which serves as the ground-truth text response for part-level constraint-aware segmentation.
% This decomposition is performed using the off-the-shelf GPT-4o API.


% After obtaining the subgoals, constraints, and object-part associations for each stage, we need to assign each frame to its corresponding stage.
% % While BridgeData V2 provides trajectory-level instructions, we require frame-level annotations for per-frame subgoals and constraints.
% %
% Since BridgeData V2 does not provide per-frame annotations, we addressed this issue by sampling pick-and-place data and leveraging the additional information~(\eg, gripper open/close states) provided by BridgeData V2 for assignment. 
% The pick-and-place task is typically divided into three stages: Approach, Grasp and Transfer, and Place, corresponding to the gripper states of open, closed, and open, respectively.
% Leveraging the characteristics of the pick-and-place task, we complete the frame-level assignment. Subfigure 2 in \cref{fig: sup data collection} illustrates a specific example of the assignment process.

% Using the obtained frame-level constraint-aware object and part information, Instance-level and part-level segmentations are performed using Grounded SAM~\cite{ren2024grounded} and Semantic SAM~\cite{li2023semantic}, respectively. 
% We conducted a sampled manual inspection of the final annotations to filter out errors and low-quality labels. Our final dataset is composed of $10,181$ trajectories with $219,356$ images.
% % using external references~(\eg, gripper open/close states) to generate $10,181$ trajectories with $219,356$ images. 
% % %
% % We employ GPT-4o to decompose trajectory instructions into subgoals, constraints, and object-part associations to generate ground-truth annotations. 
% %

% %
% % These outputs are integrated and refined through manual inspection to produce the multi-granularity dataset, which is combined with LISA's training data to fine-tune our model. More details are in Supp.~A.
% \subsection{{\mname} Training Details}
% \noindent We adopt LISA's~\cite{lai2024lisa} loss function, including the next-token prediction loss for text output, and the combination of per-pixel BCE loss with DICE loss for mask output.
% Our {\mname}-13B model is trained on an $8$ NVIDIA 80G H800 GPU for two days with a batch size of $4$.

% To ensure our model retains both dialogue and reasoning segmentation capabilities while achieving constraint-aware segmentation, our training data comprises multiple components: SemanticSeg, ReferSeg, VQA, ReasonSeg, and ConstraintSeg.
% This training data setting is inspired by LISA.
% SemanticSeg includes ADE20K, COCO-Stuff, PACO-LVIS and PASCALPart. ReferSeg includes refCLEF, refCOCO, refCOCO+, and refCOCOg. VQA includes LLaVAInstruct-150k. ConstraintSeg includes instance and part-level data.

% % We collect a small dataset to fine-tune ConSeg for each simulator. 
% The training setting described above is for the {\mname}-base model. Since the training data consists entirely of real-world scenarios, there is a significant gap between the simulation and real-world environments. 
% To address this, the {\mname} model used in the simulation experiments is a fine-tuned version, called {\mname}-ft, finetuned on a small amount of data collected from the simulator. Specifically, we collect $100$ trajectories from each simulator, sampled frames at $1$ Hz, and utilize either ground truth masks from the simulator or annotations generated using Grounded SAM and Semantic SAM.
% \highlight{Notably, we use the {\mname}-base model in real-world experiments, demonstrating the model's generalization capability across different scenarios.}


% \subsection{Element Pipeline Details}
% \label{supsubsec: element pipeline details}
% Here, we provide additional details about the Constraint Element Pipeline. After obtaining the constraint-aware object/part point clouds, we first filter out outliers. Next, we calculate the 3D spatial bounds occupied by the remaining point cloud and determine the voxel size for voxelization based on the element type.
% We then perform point cloud clustering using the DBSCAN algorithm, which has advantages over other methods, including the ability to identify clusters of arbitrary shapes, the elimination of the need to predefine the number of clusters, and its effectiveness in high-density regions.



% % Environment Setups, Policies, and Baselines

% \section{Environment Configuration}
% \label{supsec: environment configuration}

% We first provide detailed descriptions of the simulators (CLIPort~\cite{shridhar2021cliport}, Omnigibson~\cite{li2022behavior}, RLBench~\cite{james2019rlbench}) and real-world setups used in our study. 
% %
% We then discuss the low-level control policies implemented in these environments. 
% %
% Finally, we present the baselines and their implementation specific to each environment.
% %
% \highlight{Notably, our framework, {\fname}, is policy agnostic, meaning it can be adapted to any control policy without requiring any modification.}


% \subsection{Environmental Setup}


% \begin{figure*}[t]
% \centering
% \includegraphics[width=\linewidth]{fig/obs_space.pdf}
%    \caption{Environmental Setup of three simulators and one real-world setting.
%    %
%    For CLIPort~\cite{shridhar2021cliport} and OmniGibson~\cite{li2022behavior}, we provide third-person front and top views and the robot platforms are the UR5 arm and Fetch, respectively. 
%    %
%    RLBench~\cite{james2019rlbench} offers four camera views, including front left shoulder, right shoulder, and wrist views, with the robot platform being Franka equipped with a gripper. 
%    %
%    We provide a wrist and a third-person front view for the real-world setting, utilizing a UR5 robot equipped with a Leap Hand~\cite{shaw2023leap}.
%    }
% \label{fig: sup obs space}
% \end{figure*}






% The CLIPort~\cite{shridhar2021cliport} simulator\footnote{\url{https://github.com/cliport/cliport}} is a robotic manipulation benchmark to gather extensive data for imitation learning and train a language-conditioned multi-task low-level control policy.
% %
% The environment features a UR5 robotic arm with a suction cup as the end effector for pick-and-place tasks and a spatula as the end effector for pushing tasks, both operating on a black tabletop. 
% %
% We use two cameras: a third-person front view and a top view to provide comprehensive perspectives of the tabletop, as shown in \cref{fig: sup obs space}~(a).


% The OmniGibson~\cite{li2022behavior} simulator\footnote{\url{https://github.com/StanfordVL/OmniGibson}} offers a realistic setting including a physics engine capable of supporting features such as lighting rendering, gravity effects, and temperature variations impacting objects within the environment.
% %
% This platform also provides an extensive array of pre-configured scenes and objects, enabling researchers to customize setups and train mobile manipulation robots.
% %
% We select version 1.1.0 for our study.
% %
% This simulator involves a Fetch robot equipped with a gripper as the end effector, operating on a white tabletop. 
% %
% We utilize two cameras: a third-person front view and a top view to provide comprehensive perspectives of the tabletop, as shown in \cref{fig: sup obs space}~(b).


% RLBench~\cite{james2019rlbench} simulator\footnote{\url{https://github.com/stepjam/RLBench}} is a widely used benchmark for robot manipulation, featuring tasks such as articulated objects and tool use. 
% %
% Researchers can gather data and train low-level control policies using imitation learning or reinforcement learning within this environment. 
% %
% RLBench features a Franka robotic arm with a gripper as its end effector, operating on a brown tabletop. Four cameras provide comprehensive tabletop coverage, as shown in \cref{fig: sup obs space}~(c).
% %
% Additionally, RLBench uses a sampling-based motion planner for motion planning given the next predicted action/pose.


% In the real-world setup depicted in \cref{fig: sup obs space}~(d), we utilize a fixed UR5 robotic arm with a Leap Hand~\cite{shaw2023leap} as the end effector. 
% %
% Two RealSense D415 RGB-D cameras capture the scene, one mounted on the wrist and the other positioned for a third-person front view.
% %





% \begin{figure*}[t]
% \centering
% \includegraphics[width=\linewidth]{fig/cliport_task.pdf}
%    \caption{
%    CLIPort task demonstration. we present three types of tasks in our experiments, including the starting and ending frames.
%    }
% \label{fig: sup cliport task}
% \end{figure*}



% \begin{table*}[t]
% \caption{Detailed Performance in CLIPort. We report the success rate and execution time for three tasks, compared to baseline methods.}
% \centering
% \small
% \renewcommand{\arraystretch}{1.2} % 增加行间距
% \setlength{\tabcolsep}{1.5pt}
% \begin{tabular}{lc|c|ccc|ccc}
% \bottomrule[1pt]
% \multicolumn{2}{c|}{Tasks with}                  & \multicolumn{4}{c}{Success Rate(\%) $\uparrow$} & \multicolumn{3}{c}{Execution Time(s) $\downarrow$} \\
% \multicolumn{2}{c|}{disturbance}                & CLIPort & +Inner Monologue  & +DoReMi & +\textbf{Ours}  & +Inner Monologue & +DoReMi & +\textbf{Ours} \\
% \hline
%   Stack in         & $p$=0.0                   & 100.00 $\pm$ 0.00 & 100.00 $\pm$ 0.00  & 100.00 $\pm$ 0.00 & 100.00 $\pm$ 0.00    & 13.40 $\pm$ 1.82 & 13.40 $\pm$ 1.82 & 13.40 $\pm$ 1.82   \\
%   order with       & $p$=0.15                  & 56.67 $\pm$ 6.11  & 81.67 $\pm$ 6.11  & 83.33 $\pm$ 5.17 & \textbf{95.00 $\pm$ 4.00}        & 34.80 $\pm$ 3.12 & 26.00 $\pm$ 2.77 & \textbf{21.00 $\pm$ 1.75} \\
%   drop $p$         & $p$=0.3                   & 21.67 $\pm$ 8.33 & 75.00 $\pm$ 8.95  & 76.67 $\pm$ 9.52 & \textbf{88.33 $\pm$ 6.53}    & 42.80 $\pm$ 3.18 & 34.20 $\pm$ 2.73 & \textbf{25.40 $\pm$ 2.95} \\
% \hline
%   Stack in         & $q$=1                     & 90.00 $\pm$ 6.11  & 90.00 $\pm$ 6.11  & 96.67 $\pm$ 4.00 & \textbf{98.33 $\pm$ 3.27}    & 24.80 $\pm$ 4.08 & 24.60 $\pm$ 4.66 & \textbf{24.20 $\pm$ 4.65}   \\
%   order with       & $q$=2                     & 41.67 $\pm$ 7.30 & 71.67 $\pm$ 8.33  & 75.00 $\pm$ 5.17 & \textbf{83.33 $\pm$ 5.17}        & 39.40 $\pm$ 5.87 & 37.00 $\pm$ 6.29 & \textbf{29.20 $\pm$ 4.61} \\
%   noise $q$        & $q$=3                     & 15.00 $\pm$ 6.11 & 40.00 $\pm$ 8.00  & 40.00 $\pm$ 6.11 & \textbf{63.33 $\pm$ 8.33}    & 58.20 $\pm$ 4.74 & 54.20 $\pm$ 6.02 & \textbf{36.80 $\pm$ 4.61} \\
% \hline
%   \multicolumn{2}{c|}{Sweep Half the Blocks}   & 0.00 $\pm$ 0.00 & 18.33 $\pm$ 6.11  & 16.67 $\pm$ 8.95 & \textbf{75.00 $\pm$ 11.55}    & 22.00 $\pm$ 2.91 & 16.60 $\pm$ 1.33 & \textbf{16.40 $\pm$ 1.00}   \\
% \hline
%   \multicolumn{2}{l|}{Use Rope to Close}   & \multirow{2}{*}{0.00 $\pm$ 0.00} & \multirow{2}{*}{68.33 $\pm$ 9.52}  & \multirow{2}{*}{58.33 $\pm$ 18.62} & \multirow{2}{*}{\textbf{76.67 $\pm$ 6.11}}    & \multirow{2}{*}{41.60 $\pm$ 6.34} & \multirow{2}{*}{65.80 $\pm$ 7.40} & \multirow{2}{*}{\textbf{34.60 $\pm$ 2.81}}   \\
%   \multicolumn{2}{l|}{the Opening Square}   &  &   &  &     &  &  &    \\

% \bottomrule[1pt]
% \end{tabular}
% \label{tab: sup cliport}
% \end{table*}




% \subsection{Control Policy}

% In CLIPort, we use a pre-trained low-level policy the CLIPort~\cite{shridhar2021cliport} simulator provides to control the robotic arm and end effector. 
% %
% This policy can execute multi-task operations based on language instructions with RGB observations and its performance approaches perfection due to extensive imitation learning training. 
% %
% Notably, the policy is open-loop, meaning it does not adjust its actions in response to dynamic environmental changes~(\eg, it will not immediately pick up a dropped block during movement but will continue with the previously planned actions).


% In Omnigibson, We utilize ReKep~\cite{huang2024rekep} as our low-level control policy, transforming long-horizon tasks into a set of relationships between fixed keypoints at different stages.
% %
% At each stage, an optimization algorithm computes these relationships to generate actions, enabling language-conditioned closed-loop control. 
% %
% Notably, ReKep employs a pre-trained large vision model (\ie, DINOv2~\cite{oquab2023dinov2}) to process raw RGB data, extracting semantically relevant keypoints. 
% %
% This approach also serves as the compared method in our ablation study for extracting 3D points through constraint-aware segmentation, showing our superiority.



% In RLBench, we employ the Autoregressive Policy~(ARP)~\cite{zhang2024autoregressive} as the control policy, which generates the next action based on historical observations and action sequences through an autoregressive process. 
% %
% This method achieves state-of-the-art performance in the RLBench.



% In the real-world setting, We employ DexGraspNet 2.0~\cite{zhang2024dexgraspnet} as our low-level policy, which predicts the dexterous hand's grasping pose based on the scene's point cloud and facilitates the robotic arm's action trajectory through motion planning to achieve robust generalized grasping.
% %
% {Notably, DexGraspNet 2.0 is an open-loop policy, which means it does not adjust to environmental changes during action execution.} 
% %
% For example, if the target object's position shifts while the arm moves, the system does not modify its motion plan. 
% %
% Therefore, it continues to execute toward the originally intended location to complete the grasp, failing.


% \subsection{Baseline Details}

% In CLIPort, we compare three baselines: CLIPort~\cite{shridhar2021cliport}, CLIPort with Inner Monologue~\cite{huang2022inner}, and CLIPort with DoReMi~\cite{guo2023doremi}. 
% %
% We slightly modify the original implementations of these three baselines to suit our task requirements.
% %
% \textbf{(1)} For CLIPort~\cite{shridhar2021cliport}, the sole modification involves substituting the original oracle success detector with an off-the-shelf VLM (\ie, GPT-4o~\cite{achiam2023gpt}) used as a failure detector. 
% %
% This change enables the robot system to determine whether to transition to the next subgoal using image-based vision question answering~(VQA). 
% %
% Notably, CLIPort decomposes the instructions into a list of subgoals before the task begins and does not dynamically adjust or revert to previous subgoals upon detecting a failure.
% %
% \textbf{(2)} For Inner Monologue~\cite{huang2022inner}, we replicate the implementation detailed in the original literature, by employing CLIPort for the low-level policy and an off-the-shelf VLM (\ie, GPT-4o~\cite{achiam2023gpt}) as the planner. 
% %
% This pipeline determines the next subgoal based on the completed subgoals and current observations after each subgoal concludes. 
% %
% Notably, Inner Monologue queries the VLM only at the end of each subgoal, without considering events that occur during execution.
% %
% \textbf{(3)} For DoReMi~\cite{guo2023doremi}, we reproduce the implementation according to the original DoReMi paper and enhance it by replacing the VLM initially~(\ie, BLIP2~\cite{li2023blip}) used for repeated VQA-style queries during robotic execution with a more powerful VLM (\ie, GPT-4o~\cite{achiam2023gpt}). 
% %
% Additionally, we substitute its LLM, which lacks environmental awareness, with the same GPT-4o to serve as the task planner.


% In Omnigibson, we compare two baselines: ReKep~\cite{huang2024rekep} and ReKep with DoReMi~\cite{guo2023doremi}. 
% %
% \textbf{(1)} For ReKep, we directly implement it using the official codebase. 
% %
% \textbf{(2)} For DoReMi, it is implemented as described above.


% In RLBench, we compare two baselines: ReKep~\cite{huang2024rekep} and ReKep with DoReMi~\cite{guo2023doremi}. 
% %
% \textbf{(1)} For ReKep, we directly implement it using the official codebase. 
% %
% \textbf{(2)} For DoReMi, it is implemented as described above.


% For the real-world evaluation, we compare two baselines: 
% %
% DexGraspNet 2.0~\cite{zhang2024dexgraspnet} and DexGraspNet 2.0 with DoReMi~\cite{guo2023doremi}. 
% %
% \textbf{(1)} For DexGraspNet 2.0, we directly implement it using the official codebase. 
% %
% \textbf{(2)} For DoReMi, it is implemented as described above.












% \section{Evaluation Details}
% \label{supsec: evaluation details}

% In this section, we first detail the task specifications within the simulator and real-world evaluations.
% %
% Then, we introduce the disturbances introduced in each task and the evaluation metrics used. 
% %
% Finally, we report the detailed experimental results and our analyses, with additional results not included in the main text due to space constraints.


% \subsection{CLIPort}
% \label{supsubsec: cliport evaluation details}


% \begin{figure*}[t]
% \centering
% \includegraphics[width=\linewidth]{fig/omnigibson_task.pdf}
%    \caption{
%    Omnigibson task demonstration. we present three types of tasks in our experiments, including the starting and ending frames.
%    }
% \label{fig: sup omnigibson task}
% \end{figure*}



% \subsubsection{Task, Disturbance and Metric Details}



% As shown in \cref{fig: sup cliport task}, we evaluate three tasks in CLIPort:
% \textbf{(1)} ``Stack in Order'': Given blocks in red, green, and blue on a table, the robot must stack them with red at the bottom, green in the middle, and blue on top.
% %
% \textbf{(2)} ``Sweep Half the Blocks'' With $40$ blocks on the table, the robot must sweep approximately half of them (with a permissible error margin of $\pm 10\%$, \ie, $16$ to $24$ blocks) to a designated area.
% %
% \textbf{(3)} ``Use Rope to Close the Opening Square'': The robot should use a rope to enclose an open square, to enclose the area sufficiently, rather than form a perfectly closed square.




% We introduce two types of disturbances to the ``Stack in Order'' task: 
% %
% \textbf{(1)} after the suction cup grasps a block, there is a probability $p$ at each step that the block will be released, causing it to drop; 
% %
% \textbf{(2)} The predicted placement position by the policy is perturbed by a uniform noise in the range $[0,q]$ cm, potentially leading to block tower collapse.


% For each task and disturbance type, we conduct $5$ trials using different seeds, each comprising $12$ episodes.
% %
% We assess performance based on success rate and execution time, \highlight{excluding} the computational time for invoking the VLM. 
% %
% Results are reported as mean values with $95\%$ confidence intervals.
% %
% In the ``Stack in Order'' task, the robot must successfully stack the blocks in the specified order into a tower within $70$ seconds, despite the two perturbations above.
% %
% For the ``Sweep Half the Blocks'' task, the pre-trained policy aims to sweep blocks into a designated area. The robot must stop the policy once half of the blocks are in the target region. If, after $30$ seconds, the number of blocks in the area falls within the required range ($16$–$24$), the task is considered successful.
% %
% For the ``Use Rope to Close the Opening Square'' task, the pre-trained policy attempts to close an open rectangle into a perfect square using a rope. The robot must detect when the rectangle is sufficiently enclosed and immediately stop execution. Success is achieved if the robot halts within $70$ seconds, and the enclosure is complete.
% %


% \subsubsection{Detailed Experiment Results}
% In \cref{tab: sup cliport}, we present detailed results in CLIPort, including those discussed in the main text and additional results.


% In the ``Stack in Order'' task under severe interference conditions, our {\fname} shows an improvement of $18.33\%$ and $17.5\%$ in success rate over Inner Monologue~\cite{huang2022inner} and DoReMi~\cite{guo2023doremi}, respectively, while also reducing execution times by $38.7\%$ and $14.4\%$ compared to Inner Monologue and DoReMi, respectively.
% %
% % We find that utilizing code with elements enables both \textit{reactive} and \textit{proactive} failure detection, allowing for real-time identification and prevention of failure. 
% %
% % Furthermore, calculating the spatial relationships of elements through code provides superior monitoring of 3D spatial relations compared to direct image query via VLM. 
% %
% % These findings are discussed in the main text, and the processes of failure detection and recovery are shown in \cref{xxx}.
% %
% The failure detection and recovery processes are shown in \cref{fig: sup cliport demo 1} and \cref{fig: sup cliport demo 2}.



% In the ``Sweep Half the Blocks'' task, our {\fname} achieved success rates that are $4.1$ and $4.5$ times higher than those of Inner Monologue~\cite{huang2022inner} and DoReMi~\cite{guo2023doremi}, respectively. 
% %
% % This means that directly computing the 3D positions of block-representative points to verify their presence within a rectangular area offers greater precision than relying on VLMs for image interpretation, as outlined in the main text.  
% %
% However, the success rate is not very high even in distraction-free scenarios.  
% %
% This is attributed to the high density of tracking points in the scene, which increases the likelihood of confusion and tracking errors, leading to inconsistent block counts within the target area.
% %
% The completion process of the task is also illustrated in \cref{fig: sup cliport demo 3}.



% In the ``Use Rope to Close the Opening Square'' task, our approach outperforms Inner Monologue~\cite{huang2022inner} and DoReMi~\cite{guo2023doremi} by $8.34\%$ and $18.34\%$ in success rates, respectively, while also reducing execution times by $16.82\%$ and $47.43\%$ compared to Inner Monologue and DoReMi, respectively.
% %
% We find that calculating the distance between the rope ends and the opening's edges to determine closure is more accurate than directly querying a VLM with an image, allowing for earlier termination of the policy execution. 
% %
% The complete processes of the task are illustrated in \cref{fig: sup cliport demo 4}.






% \begin{figure*}[t]
% \centering
% \includegraphics[width=\linewidth]{fig/rlbench_task.pdf}
%    \caption{
%    RLBench task demonstration. we present six types of tasks in our experiments, including the starting and ending frames.
%    }
% \label{fig: sup rlbench task}
% \end{figure*}



% \subsection{OmniGibson}
% \label{supsubsec: omnigibson evaluation details}


% \subsubsection{Task, Disturbance and Metric Details}

% As shown in \cref{fig: sup omnigibson task}, in the OmniGibson environment, we evaluated three distinct tasks:
% %
% \textbf{(1)} Slot Pen: A pen placed on a desk is picked up, rotated to a near-vertical position, moved above a pen holder, and then inserted into the holder.
% %
% \textbf{(2)} Stow Book: A book located on a desk is picked up and vertically positioned on a bookshelf.
% %
% \textbf{(3)} Pour Tea: A teapot on the desk is lifted, horizontally moved above a teacup, and then tilted to pour tea into the cup.


% We introduce three types of disturbances with varying constraint elements for each task:
% %
% \textbf{(1)} Slot Pen Task: Point-level disturbances are applied as follows: (a) moving the pen while the robot is grasping it, (b) forcing the robot to release the pen mid-transfer, causing it to drop onto the table, and (c) moving the pen holder while the robot attempts to insert the pen. Despite these disturbances, the task is considered successful only if the robot can insert the pen into the holder.
% %
% \textbf{(2)} Stow Book Task: Line-level disturbances include: (a) rotating the book during the robot’s grasping process, (b) altering the book’s pose during transfer to disrupt its vertical alignment, and (c) reorienting the book horizontally after it has been placed vertically on the shelf. Success requires the robot to place the book vertically on the shelf despite these disturbances.
% %
% \textbf{(3)} Pour Tea Task: Surface-level disturbances involve: (a) tilting the container forward or backward during transfer, (b) inducing lateral tilts during movement, and (c) restoring the container to a level position during pouring. To succeed, the robot must prevent spillage and complete the pouring task under these disturbances.


% We conduct experiments on three tasks, each consisting of one no-disturbance trial and three specific-disturbance trials. Each trial was repeated 10 times, and the performance was evaluated based on success rate, execution time (\highlight{including} the computation time for invoking the VLM), and the number of tokens used.


% \subsubsection{Detailed Experiment Results}


% Specific experimental results are detailed in the main text; here, we present additional demonstrations in Sec.\ref{supsubsec: omniGibson demonstrations}.






% \subsection{RLBench}
% \label{supsubsec: rlbench evaluation details}


% \subsubsection{Task, Disturbance and Metric Details}

% As shown in \cref{fig: sup rlbench task}, in RLBench, we evaluate six tasks across three categories of manipulation:
% %
% \textbf{(1)} Articulated Object Interaction: (a) Open Drawer——Open the top drawer (b) Put in Drawer——Open the drawer and place an item into the open drawer.
% %
% \textbf{(2)} Rotational Manipulation: (a) Screw Bulb——Screw in the red light bulb. (b) Turn Tap——Turn the left tap.
% %
% \textbf{(3)} Tool Use: (a) Drag Stick——Use a stick to drag the cube onto the red target. (b) Sweep to Dustpan——Sweep dirt into the tall dustpan.

% In RLBench, we avoid introducing additional disturbances, as its control policy naturally generates diverse failures to validate the effectiveness of our framework.

% For each task, we conducted $1,000$ episodes with each episode having a length of $25$. The tasks were evaluated based on the average success rate.

% \subsubsection{Detailed Experiment Results}


% % 
% % 值得注意的是，尽管我们的训练数据中没有任何有关铰链物体的数据，
% \highlight{Code with elements can generalize better to monitor diverse tasks.}
% %
% \highlight{Notably, despite our training data lacking information on articulated objects at both the instance and part levels, our method effectively handles them, accurately segmenting parts such as drawer handles}. 
% %
% In the ``Open Drawer'' task, {\fname} achieves a $98.1\%$ success rate, significantly outperforming DRM's $90.6\%$.
% %
% For ``Put in Drawer'', CaM reaches $98.3\%$, surpassing DRM's $87.7\%$ by $10.6$ percentage points. 
% %
% \highlight{We attribute this generalization to two factors: \textbf{(1)} the inherent prior world knowledge of extensively pre-trained VLMs (\eg, SAM, LLaVA), which enables generalization to unseen tasks; and \textbf{(2)} our minimalist scheme that abstracts articulated objects into geometric components via constraint elements, ignoring irrelevant details, enhancing the generalizability.}


% We also demonstrate our method on additional unseen tasks, such as rotational manipulation and tool use, where it consistently outperforms baseline methods. 

% \begin{table*}[t]
% \caption{Performance in RLBench. We report the success rate, compared to baseline methods.}
% \small
% \centering
% % \setlength{\tabcolsep}{2.5pt}
% \begin{tabular}{l|c|cc|cc|cc}
% \bottomrule[1pt]
% \multirow{2}{*}{Method}        &   Avg.                     
%                                & \multicolumn{2}{c|}{Articulated Object} 
%                                & \multicolumn{2}{c|}{Tool-Use} 
%                                & \multicolumn{2}{c}{Tool-Use}  
%                                \\
% \cline{3-8}
%                                &  Success  Rate~(\%) $\uparrow$                 &  Open Drawer    &   Put in  Drawer                   & Screw Bulb  & Turn  Tap               &  Drag Stick     &   Sweep to  Dustpan      \\
% \hline

%  RVT2~\cite{goyal2024rvt2}          &89.83         &90.3     &97.6    &86.6   &91.0   &93.8     &79.7 \\  
% ARP~\cite{zhang2024autoregressive}  &91.27         &93.9     &91.0    &86.4   &96.6   &88.1     &91.6 \\        

% \hline

% ~~+DRM~\cite{guo2023doremi}         &87.97         &90.6     &87.7   &83.1   &93.3    &84.8     &88.3 \\               
% ~~\textbf{+Ours}                    &\textbf{97.08}         & \textbf{98.1}     &\textbf{98.3}   &\textbf{97.5}   &\textbf{97.9}     &\textbf{95.6}     &\textbf{94.0} \\                          

% \bottomrule[1pt]
% \end{tabular}
% \label{tab: rlbench}
% \end{table*}




% \subsection{Real-world Evaluation}
% \label{supsubsec: real-world evaluation details}

% \begin{table*}[t]
% \caption{Detailed Performance of Single Pick \& Place. We report the success rate and execution time. DGN donates DexGraspNet 2.0~\cite{zhang2024dexgraspnet}.}
% \centering
% \small
% % \setlength{\tabcolsep}{3pt}
% \begin{tabular}{l|cc|c|cc|cc}
% \bottomrule[1pt]
% Tasks with         & Object   & Object  & \multicolumn{3}{c}{Success Rate(\%) $\uparrow$} & \multicolumn{2}{c}{Execution Time(s) $\downarrow$} \\
% disturbance        & types    & Name    & DGN  & +DoReMi & +\textbf{Ours}   & +DoReMi & +\textbf{Ours} \\

% \hline
%  Pick \& Place with         & \multirow{3}{*}{Deformable}   & Toy Loopy   & 0.00  & 80.00 & \textbf{100.00}        & 64.91 $\pm$ 2.83 & \textbf{46.02$\pm$  3.11}   \\
%  the objects being          &    & Toy Dog   & 0.00  & 80.00 & \textbf{100.00}        & 60.68 $\pm$ 4.00 & \textbf{47.06 $\pm$ 3.24}   \\
%  moved during               &    & Toy Rabbit   & 0.00  & 90.00 & \textbf{90.00}        & 59.83 $\pm$ 1.82 & \textbf{45.77 $\pm$ 2.03}   \\
%                             \cline{2-8}
%  grasping                   & \multirow{3}{*}{Transparent}  & Beverage Bottle   & 0.00  & 60.00 & \textbf{100.00}        & 69.97 $\pm$ 7.89 & \textbf{47.61 $\pm$ 2.58} \\
%                             &   & Glass Cup   & 0.00  & 70.00 & \textbf{90.00}        & 76.99 $\pm$ 4.60 & \textbf{48.32 $\pm$ 3.22} \\
%                             &   & Shampoo Bottle   & 0.00  & 70.00 & \textbf{90.00}        & 70.91 $\pm$ 5.68 & \textbf{48.31 $\pm$ 3.08} \\
%                             \cline{2-8}
%                             & \multirow{3}{*}{Small Rigid}  & Apple Model   & 0.00  & 80.00 & \textbf{100.00}        & 64.65 $\pm$ 4.34 & \textbf{45.39 $\pm$ 0.71} \\
%                             &   & Pear Model   & 0.00  & 90.00 & \textbf{90.00}         & 67.11 $\pm$ 1.10 & \textbf{45.48 $\pm$ 1.01} \\
%                             &   & Peach Model   & 0.00  & 70.00 & \textbf{90.00}        & 65.48 $\pm$ 2.90 & \textbf{45.37 $\pm$ 0.64} \\
%                             \cline{2-8}
%                             & \multirow{3}{*}{Large Geometric} & Plate & 0.00  & 80.00 & \textbf{100.00}        & 69.86 $\pm$ 2.64 & \textbf{45.18 $\pm$ 0.65} \\
%                             &  & Ball & 0.00  & 90.00 & \textbf{100.00}        & 67.43 $\pm$ 2.63 & \textbf{45.37 $\pm$ 0.70} \\
%                             &  & Pyramid & 0.00  & 90.00 & \textbf{90.00}        & 69.14 $\pm$ 3.32 & \textbf{45.42 $\pm$ 0.72} \\
% \hline
%  Pick \& Place with         & \multirow{3}{*}{Deformable}   & Toy Loopy   & 0.00  & 80.00 & \textbf{90.00}        & 69.29 $\pm$ 4.87 & \textbf{60.86 $\pm$ 3.41}   \\
%  the objects being          &    & Toy Dog   & 0.00  & 70.00 & \textbf{100.00}        & 66.09 $\pm$ 2.99 & \textbf{63.12 $\pm$ 3.75}   \\
%  removed during             &    & Toy Rabbit   & 0.00  & 80.00 & \textbf{90.00}        & 70.86 $\pm$ 4.56 & \textbf{63.40 $\pm$ 3.88}   \\
%                             \cline{2-8}
%  movement                   & \multirow{3}{*}{Transparent}  & Beverage Bottle   & 0.00  & 50.00 & \textbf{90.00}        & 77.90 $\pm$ 2.89 & \textbf{61.97$\pm$  3.90} \\
%                             &   & Glass Cup   & 0.00  & 70.00 & \textbf{90.00}        & 70.00 $\pm$ 3.46 & \textbf{63.22 $\pm$ 4.35} \\
%                             &   & Shampoo Bottle   & 0.00  & 60.00 & \textbf{90.00}        & 60 $\pm$ 4.28 & \textbf{63.00 $\pm$ 3.81} \\
%                             \cline{2-8}
%                             & \multirow{3}{*}{Small Rigid}  & Apple Model   & 0.00  & 70.00 & \textbf{90.00}        & 70.21 $\pm$ 4.30 & \textbf{63.71 $\pm$ 3.91} \\
%                             &   & Pear Model   & 0.00  & 60.00 & \textbf{100.00}        & 72.70 $\pm$ 4.84 & \textbf{58.61$\pm$  2.41} \\
%                             &   & Peach Model   & 0.00  & 60.00 & \textbf{90.00}        & 66.48 $\pm$ 3.32 & \textbf{59.19 $\pm$ 2.59} \\
%                             \cline{2-8}
%                             & \multirow{3}{*}{Large Geometric} & Plate & 0.00  & 90.00 & \textbf{100.00}        & 72.00 $\pm$ 2.77 & \textbf{59.21 $\pm$ 2.61} \\
%                             &  & Ball & 0.00  & 70.00 & \textbf{100.00}        & 70.92 $\pm$ 3.37 & \textbf{61.57 $\pm$ 3.80} \\
%                             &  & Pyramid & 0.00  & 70.00 & \textbf{90.00}        & 73.83 $\pm$ 2.82 & \textbf{60.25 $\pm$ 3.25} \\
% \bottomrule[1pt]
% \end{tabular}
% \label{tab: sup hand 1}
% \end{table*}

% \subsubsection{Task, Disturbance and Metric Details}
% We conduct real-world evaluations on two tasks:
% %
% \textbf{(1)} Simple Pick \& Place: The robot should pick and place objects within $70$ seconds. 
% %
% We include four kinds of objects: Deformable, Transparent, Small Rigid, and Large Geometric, with three objects in each category. 
% %
% The deformable objects are Loopy,  Dog, and  Rabbit toys, which undergo deformation when grasped by the dexterous hand.
% %
% The transparent objects are a clear beverage bottle, a transparent glass, and a clear shampoo bottle. 
% %
% The small rigid objects consist of apple, pear, and peach models, while the large geometric objects include a large plate, ball, and pyramid.
% %
% \textbf{(2)} Reasoning Pick \& Place: In cluttered scenes, the robot must perform long-horizon tasks where the instructions contain ambiguous terms (\eg, ``animals'' or ``fruits'' without specifying particular types). 
% %
% Specifically, the tasks are: (a) ``Clear all objects on the table except for \underline{animals}'', and (b) "Grasp the \underline{animals} according to their distances to \underline{fruits}, from nearest to farthest'', with ambiguous terms underlined.




% For both tasks, we introduce two identical disturbances:
% %
% \textbf{(1)} Moving the object during the robot's grasping.
% %
% \textbf{(2)} Removing the object from the robot's dexterous hand during movement after grasping.



% For each task, and each object involved in Simple Pick \& Place, we conduct 10 trials.
% %
% For each long-horizon task in Reasoning Pick \& Place, we also conduct 10 trials.
% %
% We evaluate performance based on success rate and execution time, \highlight{including} the computational time invoking the VLM.
% %
% Results are reported as mean values with $95\%$ confidence intervals.
% %
% For the Simple Pick \& Place, the robot has only one opportunity to autonomously release the object held in its gripper at a designated location. 
% %
% Any disturbance the robot encounters allows for a return and reattempt at grasping if the robot successfully detects it. 
% %
% Success is defined as meeting these conditions within $90$ seconds.
% %
% For the Reasoning Pick \& Place task, the robot must clear all objects on the table except for animals within $4$ minutes for ``Clear all objects on the table except for animals''. 
% %
% In the task ``Grasp the animals according to their distances to fruits, from nearest to farthest'', the robot must sequentially grasp the animals in the correct order within $2$ minutes, despite human-induced distractions such as moving animals or fruits.
% %
% \highlight{Notably, this task is particularly challenging because the robot operates under an open-loop policy, preventing it from using closed-loop feedback to handle the dynamic distances between fruits and animals caused by external disturbances.
% %
% Therefore, a failure detection framework is necessary to enable both \textit{reactive} and \textit{proactive} real-time detection with high precision, monitoring the distance changes and adjusting the grasping sequence accordingly.}


% \subsubsection{Detailed Experiment Results}

% In \cref{tab: sup hand 1}, we present detailed results of Simple Pick \& Place.
% %
% {\fname} achieves success rates surpassing DoReMi by $20.4\%$ when handling different kinds of objects.
% %
% We show real-world demonstrations of Simple Pick \& Place and Reasoning Pick \& Place in Sec.~\ref{supsubsec: real-world demonstrations}.


% \section{Limitations and Future Work}
% \label{supsec: more discussion}

% Despite promising results, our approach has several limitations.
% %
% First, using Visual Language Models (VLMs)—such as off-the-shelf GPT for code generation and constraint-aware segmentation models—inevitably leads to hallucination issues. Even with minimized VLM usage, inaccuracies in code generation and biases in segmentation may persist. Integrating more relevant knowledge via methods like Retrieval-Augmented Generation (RAG)~\cite{lewis2020retrieval} or reducing multimodal large language model (MLLM) hallucinations~\cite{MinerviniAHD2024} could alleviate these problems.
% %
% Second, while we unify reactive and proactive failure detection as spatio-temporal constraint satisfaction problems and propose constraint elements for simplified real-time, high-precision monitoring, the constraint element representation has limitations:
% %
% (1) It primarily focuses on failures detectable through explicit displacement and rotation, rendering it less effective for force-direction-related failures without noticeable displacement—for example, a robotic gripper failing to open a drawer due to incorrect force application.
% %
% (2) The simplified representation abstracts objects and minimizes irrelevant visual details for efficient failure detection but may overlook critical visual cues and multimodal inputs, such as flowing water or audible sounds from a partially closed faucet, which are ignored in our current framework.
% %
% Thus, exploring more robust representations that balance real-time precision with minimal information loss or integrate richer multimodal inputs is a promising direction for future research.

% \section{More Demonstrations and Prompts}
% \label{supsec: more demonstrations and prompts}

% This section presents additional demonstrations, including simulations and real-world scenarios of failure detection and recovery, as well as constraint-aware segmentation results and prompts.



% \subsection{CLIPort}
% \label{supsubsec: cliport demonstrations}

% % 这里我们展示了 CLIPort 中三个任务 ``Stack in Order'' ``Sweep Half the Blocks'' ``Use Rope to Close the Opening Square'' 的 demonstrations

% Here, we present demonstrations of three tasks in CLIPort: ``Stack in Order'', ``Sweep Half the Blocks'', and ``Use Rope to Close the Opening Square''.


% % \cref{fig: sup cliport demo 1} 展示了 ``Stack in Order'' 这个task 面临policy预测的放置位置会受到uniform [0,q] cm 的干扰的情况下，我们的框架如何 failure detection 和并辅助 recovery的。

% \cref{fig: sup cliport demo 1} demonstrates how our framework detects failures and assists in recovery when the placement positions predicted by the policy for the ``Stack in Order'' task are subject to a uniform $[0,q]$ cm interference.

% % \cref{fig: sup cliport demo 2} 展示了 ``Stack in Order'' 这个task 面临每一步都有p的概率会方块被机器人的吸盘释放而掉落的情况下，我们的框架如何 failure detection 和并辅助 recovery的。

% \cref{fig: sup cliport demo 2} illustrates how our framework performs failure detection and aids in recovery when, in the ``Stack in Order'' task, there is a probability \( p \) that blocks will fall due to being released by the robot's suction cup at each step.


% % \cref{fig: sup cliport demo 3} 展示了 ``Sweep Half the Blocks'' 这个task，我们框架可以快速对指定区域内的方块计数，并及时停止policy执行以成功完成任务，而DoReMi无法及时停止policy执行，导致任务失败。

% \cref{fig: sup cliport demo 3} shows the ``Sweep Half the Blocks'' task, where our framework precisely counts the blocks within a specified area and timely halts the policy execution to complete the task. In contrast, DoReMi~\cite{guo2023doremi} fails to stop the policy execution in time, leading to task failure.


% % \cref{fig: sup cliport demo 4} 展示了 ``Use Rope to Close the Opening Square'' 这个task，我们框架可以有效地发现开口方块被绳子闭合，并及时停止policy执行以成功完成任务，而DoReMi无法及时停止policy执行，导致虽然最后成功闭合，但是执行时间超时，导致最终任务失败。


% \cref{fig: sup cliport demo 4} depicts the ``Use Rope to Close the Opening Square'' task. Our framework effectively detects when the rope closes the opening square and promptly stops the policy execution to complete the task successfully. Conversely, DoReMi fails to halt the policy execution on time; although it eventually succeeds in closing the opening, the excessive execution time results in task failure.

% \begin{figure*}[t]
% \centering
% \includegraphics[width=\linewidth]{fig/cliport_demo_1.pdf}
%    \caption{
%    Demonstration of ``Stack in Order''. We show how our framework detects failures and assists in recovery when the placement positions predicted by the policy for the ``Stack in Order'' task are subject to a uniform $[0,q]$ cm interference. Red boxes indicate the occurrence of failures, while green boxes signify successful task execution.
%    }
% \label{fig: sup cliport demo 1}
% \end{figure*}

% \begin{figure*}[t]
% \centering
% \includegraphics[width=\linewidth]{fig/cliport_demo_2.pdf}
%    \caption{
%    Demonstration of ``Stack in Order''. We show how our framework performs failure detection and aids in recovery when, in the ``Stack in Order'' task, there is a probability \( p \) that blocks will fall due to being released by the robot's suction cup at each step. Red boxes indicate the occurrence of failures, while green boxes signify successful task execution.
%    }
% \label{fig: sup cliport demo 2}
% \end{figure*}

% \begin{figure*}[t]
% \centering
% \includegraphics[width=\linewidth]{fig/cliport_demo_3.pdf}
%    \caption{
%    Demonstration of ``Sweep Half the Blocks'' and comparison to baseline. We show our framework can precisely count the blocks within a specified area and timely halts the policy execution to complete the task. In contrast, DoReMi~\cite{guo2023doremi} fails to stop the policy execution in time, leading to task failure. Red boxes indicate the occurrence of failures, while green boxes signify successful task execution.
%    }
% \label{fig: sup cliport demo 3}
% \end{figure*}


% \begin{figure*}[t]
% \centering
% \includegraphics[width=\linewidth]{fig/cliport_demo_4.pdf}
%    \caption{
%    Demonstration of ``Use Rope to Close the Opening Square'' and comparison to baseline. We show that our framework effectively detects when the rope closes the opening square and promptly stops the policy execution to complete the task successfully. Conversely, DoReMi fails to halt the policy execution on time; although it eventually succeeds in closing the opening, the excessive execution time results in task failure. Red boxes indicate the occurrence of failures, while green boxes signify successful task execution.
%    }
% \label{fig: sup cliport demo 4}
% \end{figure*}


% \subsection{OmniGibson}
% \label{supsubsec: omniGibson demonstrations}

% As shown in \cref{fig: sup omnigibson demo 1}, \cref{fig: sup omnigibson demo 2} and \cref{fig: sup omnigibson demo 3}, we show how our framework detects failures and assists in recovery when facing point-, line- and surface -level disturbances. 



% \begin{figure*}[t]
% \centering
% \includegraphics[width=\linewidth]{fig/omnigibson_demo_1.pdf}
%    \caption{
%    Demonstration of ``Slot Pen''. We show how our framework detects failures and assists in recovery when facing point-level disturbances. Red boxes indicate the occurrence of failures, light green indicates the recovery with subgoal success and dark green boxes signify successful task execution.
%    }
% \label{fig: sup omnigibson demo 1}
% \end{figure*}


% \begin{figure*}[t]
% \centering
% \includegraphics[width=\linewidth]{fig/omnigibson_demo_2.pdf}
%    \caption{
%    Demonstration of ``Stow Book''. We show how our framework detects failures and assists in recovery when facing line-level disturbances. Red boxes indicate the occurrence of failures, light green indicates the recovery with subgoal success and dark green boxes signify successful task execution.
%    }
% \label{fig: sup omnigibson demo 2}
% \end{figure*}


% \begin{figure*}[t]
% \centering
% \includegraphics[width=\linewidth]{fig/omnigibson_demo_3.pdf}
%    \caption{
%    Demonstration of ``Pour Tea''. We show how our framework detects failures and assists in recovery when facing surface-level disturbances. Red boxes indicate the occurrence of failures, light green indicates the recovery with subgoal success and dark green boxes signify successful task execution.
%    }
% \label{fig: sup omnigibson demo 3}
% \end{figure*}

% \subsection{Real-world Evaluation}
% \label{supsubsec: real-world demonstrations}



% % \cref{fig: sup real demo} 展示了 ``Clear all objects on table except for animals.'' 这个task，我们框架实现了 reactive failure detection~(\eg, 在人类从机械臂手中remove物体后 detect unexpected failure)和proactive failure detection~(\eg, 在机械臂抓取的过程中发现抓取的目标物体移动从而prevent foreseeable failure)，有效提供了任务的成功率以及减少任务执行时间。

% \cref{fig: sup real demo} demonstrates the task ``Clear all objects on the table except for animals'', where our framework achieves both reactive failure detection (\eg, detecting unexpected failures when humans remove objects from the robot's grasp) and proactive failure detection (\eg, identifying target object movement during grasping to prevent foreseeable failures). 
% %
% This effectively enhances the task success rate and reduces the execution time.



% \begin{figure*}[t]
% \centering
% \includegraphics[width=\linewidth]{fig/real_demo.pdf}
%    \caption{
%    Demonstration of ``Clear all objects on the table except for animals''. We show that our framework achieves both reactive failure detection (\eg, detecting unexpected failures when humans remove objects from the robot's grasp) and proactive failure detection (\eg, identifying target object movement during grasping to prevent foreseeable failures). 
%     %
%     This effectively enhances the task success rate and reduces the execution time.
%    }
% \label{fig: sup real demo}
% \end{figure*}

% \subsection{Constraint-aware segmentation}

% % 这里我们展示了更多的有关 constraint-aware segmentation的结果，包括instance 和 part level的结果。为了展示泛化性，我们选用了out-or-distrubtion（OOD）的数据，包括 REFLECT的RoboFail Dataset, Open6DOF benchmark的 dataset, 以及 RT-1 dataset。同时我们也额外展示了Omnigibson仿真中的分割结果。

% As shown in \cref{fig: sup conseg robofail}, \cref{fig: sup conseg open6dor}, \cref{fig: sup conseg rt1}, and \cref{fig: sup conseg omni} we present additional results on constraint-aware segmentation, including instance and part-level results. 
% %
% \highlight{To demonstrate generalizability, we utilize out-of-distribution (OOD) data, including the RoboFail Dataset from REFLECT~\cite{liu2023reflect}, datasets from the Open6DOF benchmark~\cite{dingopen6dor}, and the RT-1 dataset~\cite{brohan2022rt}.} Additionally, we showcase segmentation results from the OmniGibson.


% \begin{figure*}[t]
% \centering
% \includegraphics[width=\linewidth]{fig/supp_conseg_robofail.pdf}
%    \caption{
%    Visualization of constraint-aware segmentation for the RoboFail Dataset~\cite{liu2023reflect}. This dataset is not included in the training data.
%    }
% \label{fig: sup conseg robofail}
% \end{figure*}


% \begin{figure*}[t]
% \centering
% \includegraphics[width=0.9\linewidth]{fig/supp_conseg_open6dor.pdf}
%    \caption{
%    Visualization of constraint-aware segmentation for the Open6DOF~\cite{dingopen6dor}. This dataset is not included in the training data.
%    }
% \label{fig: sup conseg open6dor}
% \end{figure*}


% \begin{figure*}[t]
% \centering
% \includegraphics[width=\linewidth]{fig/supp_conseg_rt1.pdf}
%    \caption{
%    Visualization of constraint-aware segmentation for the RT-1 dataset~\cite{brohan2022rt}. This dataset is not included in the training data.
%    }
% \label{fig: sup conseg rt1}
% \end{figure*}


% \begin{figure*}[t]
% \centering
% \includegraphics[width=\linewidth]{fig/supp_conseg_omnigibson.pdf}
%    \caption{
%    Visualization of constraint-aware segmentation for the Omnigibsom simulator. 
%    % This dataset is not included in the training data.
%    }
% \label{fig: sup conseg omni}
% \end{figure*}
% \subsection{Prompts}

% As illustrated in \cref{fig: sup prompt}, we detail the prompt used to invoke an off-the-shelf VLM, \ie, GPT-4o~\cite{achiam2023gpt}, to generate Python code for monitoring.


% \begin{figure*}[t]
% \centering
% \includegraphics[width=\linewidth]{fig/prompt.pdf}
%    \caption{
%    Prompt of monitor code generation. We use this prompt, combined with additional task instructions, the current subgoal, and images from two perspectives, to enable an off-the-shelf VLM, \ie, GPT-4o~\cite{achiam2023gpt}, to generate Python code for monitoring.
%    }
% \label{fig: sup prompt}
% \end{figure*}

% \newpage
% \clearpage
% {
%     \small
%     \bibliographystyle{ieeenat_fullname}
%     \bibliography{main}
% }

% \end{document}
